# Supplementary material for: Single-cell Bayesian deconvolution
Source: arXiv:2202.06325 ancillary file (2023-06-11)
Supplement: Supplementary file 1 [file supplementary.pdf]

# Supplementary Text: Single-cell Bayesian deconvolution

Gabriel Torregrossa<sup>1</sup>, David Oriola<sup>2</sup>, Vikas Trivedi<sup>2,3</sup>, Jordi Garcia-Ojalvo<sup>1</sup>

<sup>1</sup>Department of Medicine and Life Sciences, Universitat Pompeu Fabra, 08003 Barcelona, Spain

<sup>2</sup>EMBL Barcelona, Dr. Aiguader 88, 08003 Barcelona, Spain

<sup>3</sup>EMBL Heidelberg, Developmental Biology Unit, 69117 Heidelberg, Germany

## Contents

|                                                              |           |
|--------------------------------------------------------------|-----------|
| <b>S1 Biological statement of the problem</b>                | <b>2</b>  |
| <b>S2 Mathematical statement of the problem</b>              | <b>2</b>  |
| <b>S3 Prior distributions</b>                                | <b>4</b>  |
| S3.1 MCMC priors . . . . .                                   | 4         |
| S3.2 Nested-sampling priors . . . . .                        | 5         |
| <b>S4 Posterior exploration</b>                              | <b>6</b>  |
| S4.1 MCMC sampling . . . . .                                 | 6         |
| S4.1.1 Default initial conditions for the sampling . . . . . | 10        |
| S4.1.2 Sampling identifiability and assessment . . . . .     | 11        |
| S4.2 Nested sampling . . . . .                               | 11        |
| S4.3 Sampler selection . . . . .                             | 12        |
| <b>S5 Modifications for the gamma basis</b>                  | <b>13</b> |
| <b>S6 Efficiency assessment</b>                              | <b>15</b> |
| <b>References</b>                                            | <b>16</b> |
| <b>Supplementary figures</b>                                 | <b>17</b> |

## S1 Biological statement of the problem

Flow cytometry provides us with measurements of a target signal  $T$  in large numbers of single cells. The target signal is emitted by a fluorophore that reports on the abundance (or activity) of a protein of interest within each cell. This signal is affected by autofluorescence (which can be considered a source of noise) produced by elements of the cell other than the fluorophore. Due to the noise, the total signal  $C$  measured by the device is not directly  $T$ , but

$$C = T + \xi \quad (\text{S1})$$

We are interested in the case in which we cannot measure the signal  $C$  and the noise  $\xi$  independently in the same cell, and thus  $T$  in that cell cannot be calculated trivially via Eq. (S1). This limitation is typical of flow cytometry experiments, in which cells can only be measured once. In this case, the only information that can be extracted from the device consists of the distributions of the measured signal,  $p_c$ , and of the background noise by itself,  $p_\xi$  (by measuring cells without fluorophore), over large populations of cells (tens of thousands in a typical flow cytometry run). We can assume the samples to be independent and identically distributed (iid).

If  $T$  and  $\xi$  are independent from each other, the distributions defined above are related to one another by means of a convolution:

$$p_c(C) = \int_0^\infty \int_0^\infty p_T(T) p_\xi(\xi) \delta(C - (T + \xi)) d\xi dT = \int_0^\infty p_T(C - \xi) p_\xi(\xi) d\xi =: (p_T * p_\xi)(C) \quad (\text{S2})$$

In what follows we describe a method to extract the distribution  $p_T$  of the target variable  $T$  from the observed distributions of  $C$  and  $\xi$  via a deconvolution of Eq. (S2). The method is applicable to any measurement technique that provides distributions of a signal that is affected by noise.

## S2 Mathematical statement of the problem

Since we do not know the exact underlying distributions, we model them as finite mixtures of basis functions. For the sake of concreteness, we consider for the moment normal basis functions; in Section S5 below we will extend our approach to the case of gamma basis functions.

The Gaussian mixture models for the target and the noise distributions can be represented as

$$p(T|\boldsymbol{\omega}^T, \boldsymbol{\mu}^T, \mathbf{v}^T) = \sum_{i=1}^{K_T} \omega_i^T \mathcal{N}(T|\mu_i^T, v_i^T) \quad (\text{S3a})$$

$$p(\xi|\boldsymbol{\omega}^\xi, \boldsymbol{\mu}^\xi, \mathbf{v}^\xi) = \sum_{i=1}^{K_\xi} \omega_i^\xi \mathcal{N}(\xi|\mu_i^\xi, v_i^\xi), \quad (\text{S3b})$$

where  $\mathcal{N}(x|\mu, v)$  denotes a normal distribution on the variable  $x$ , with mean  $\mu$  and variance  $v$ .  $K_T$  and  $K_\xi$  represent the number of bases used to describe each distribution,  $\boldsymbol{\omega} = \{\omega_i : i = 1 \dots K\}$  are their weights, and  $\boldsymbol{\mu} = \{\mu_i : i = 1 \dots K\}$  and  $\mathbf{v} = \{v_i : i = 1 \dots K\}$  are their characteristic parameters. Note that we have removed the subindices from the distributions of the target and the noise, since according to the mixture representation,  $p_T$  and  $p_\xi$  depend exclusively on the parameters defined above.

The mixture decomposition defined in Eqs. (S3) allows for a flexible and robust representation of unknown and generic distributions. Moreover, exploiting the fact that the convolution of two Gaussians is still a Gaussian, we have an analytical expression for the distribution of the total variable  $C$ :

$$p(c|\boldsymbol{\phi}^T, \boldsymbol{\phi}^\xi) = \sum_{i=1}^{K_T} \sum_{j=1}^{K_\xi} \omega_j^T \omega_j^\xi \mathcal{N}\left(c \middle| \mu_i^T + \mu_j^\xi, v_i^T + v_j^\xi\right), \quad (\text{S4})$$

where  $\boldsymbol{\phi}^T = \{\boldsymbol{\omega}^T, \boldsymbol{\mu}^T, \mathbf{v}^T\}$  and  $\boldsymbol{\phi}^\xi = \{\boldsymbol{\omega}^\xi, \boldsymbol{\mu}^\xi, \mathbf{v}^\xi\}$  represent all the parameters of the target and noise distributions, from which we can parametrize the distribution of the total measured signal. We note that the combined normal basis function  $\mathcal{N}$  in Eq. (S4) above is invariant under changes in the individual basis functions of  $T$  and  $\xi$ , provided the sum of means,  $\mu^T + \mu^\xi$ , and variances,  $v^T + v^\xi$ , are constant.

As discussed in the main text, according to Bayes' rule, the posterior distribution that represents the probability of the parameters given the data is

$$p(\boldsymbol{\phi}^T, \boldsymbol{\phi}^\xi | \mathbf{c}, \boldsymbol{\xi}) \propto \left[ p(\mathbf{c} | \boldsymbol{\phi}^T, \boldsymbol{\phi}^\xi) p(\boldsymbol{\xi} | \boldsymbol{\phi}^\xi) \right] \left[ p(\boldsymbol{\omega}^T) p(\boldsymbol{\phi}^\xi) p(\boldsymbol{\mu}^T) p(\boldsymbol{\mu}^\xi) p(\mathbf{v}^T) p(\mathbf{v}^\xi) \right], \quad (\text{S5})$$

where  $\mathbf{c} = \{c_i : i = 1 \dots N_c\}$  and  $\boldsymbol{\xi} = \{\xi_i : i = 1 \dots N_\xi\}$  represent the samples of the total signal and noise, respectively. In Eq. (S5), the first bracket on the right-hand side corresponds to the likelihood, namely the joint probability of observing the data given the parameters, which we can redefine as

$$\mathcal{L} = p(\mathbf{c} | \boldsymbol{\phi}^T, \boldsymbol{\phi}^\xi) p(\boldsymbol{\xi} | \boldsymbol{\phi}^\xi) = \prod_i^{N_c} p(c_i | \boldsymbol{\phi}^T, \boldsymbol{\phi}^\xi) \prod_j^{N_\xi} p(\xi_j | \boldsymbol{\phi}^\xi), \quad (\text{S6})$$

The form of the likelihood (S6) breaks the symmetry between the target and noise signals, and thus lifts the above-mentioned degeneracy between their parameters exhibited by Eq. (S4). The second bracket in

the right-hand side of Eq. (S5), in turn, corresponds to the prior distributions of all the parameters of the problem, which we define in what follows.

### S3 Prior distributions

For the vast majority of deconvolution problems, no prior information exists on the values of the parameters describing the distributions involved. Thus here we choose priors as vague as possible, provided they fulfill certain requirements, both formal (they should lead to a proper posterior distribution) and computational (they should make the sampling efficient by limiting the exploration space). To comply with these requirements, our prior specification will depend on the sampling method that we use to explore the posterior distribution. As we will see in Sec. S4, we use two sampling approaches, namely a Markov chain Monte Carlo (MCMC) method and nested sampling (NS). In what follows, we describe the prior distributions that we use with each approach.

#### S3.1 MCMC priors

The MCMC method requires that we use a set of proper priors [1] for the model to converge on an adequate posterior distribution. To that end, we choose normal distributions as priors for the means:

$$p(\mu_i^T) = \mathcal{N}(\mu_i^T | \mu_{\text{prior}}^T, v_{\text{prior}}^T) \quad (\text{S7a})$$

$$p(\mu_i^\xi) = \mathcal{N}(\mu_i^\xi | \mu_{\text{prior}}^\xi, v_{\text{prior}}^\xi) \quad (\text{S7b})$$

The hyperprior parameters are defined using heuristics from the datasets:

$$\mu_{\text{prior}}^T = \text{mean}(\mathbf{c}) - \text{mean}(\boldsymbol{\xi}) \quad v_{\text{prior}}^T = s \text{ var}(\mathbf{c}) \quad (\text{S8a})$$

$$\mu_{\text{prior}}^\xi = \text{mean}(\boldsymbol{\xi}) \quad v_{\text{prior}}^\xi = s \text{ var}(\boldsymbol{\xi}) \quad (\text{S8b})$$

where  $\mathbf{c}$  and  $\boldsymbol{\xi}$  are the datasets of the total signal and the noise, respectively. We also introduce a parameter  $s > 1$  as an expansion factor to avoid underestimating the variance of the distributions.

As priors for the variances we choose gamma distributions, defined as  $\Gamma(x|\theta, k) \propto x^{k-1} \exp(-x/\theta)$ , which avoid divergent solutions with zero variance for an appropriate choice of parameters:

$$p(v_i^T) = \Gamma(v_i^T | \theta_{\text{prior}}^T, k_{\text{prior}}^T) \quad (\text{S9a})$$

$$p(v^\xi) = \Gamma(v^\xi | \theta_{\text{prior}}^\xi, k_{\text{prior}}^\xi) \quad (\text{S9b})$$

The hyperprior parameters are again chosen using heuristics:

$$\theta_{\text{prior}}^T = s \text{ var}(\mathbf{c}) \quad k_{\text{prior}}^T = 1.1 \quad (\text{S10a})$$

$$\theta_{\text{prior}}^\xi = s \text{ var}(\boldsymbol{\xi}) \quad k_{\text{prior}}^\xi = 1.1 \quad (\text{S10b})$$

The values of  $k_{\text{prior}}^T$  and  $k_{\text{prior}}^\xi$  are chosen by hand so that the probability around zero variance is null, while keeping the possibility of small variance values. A more detailed tuning could be performed on these hyperparameters, but we consider that the choice (S10) covers a wide spectrum of length scales.

Given that the basis functions have unit area, the weight distributions must fulfill the following constraint:

$$\sum_i^{K_T} \omega_i^T = \sum_i^{K_\xi} \omega_i^\xi = 1 \quad (\text{S11})$$

A natural prior for the weights is the Dirichlet distribution:

$$p(\boldsymbol{\omega}) = \text{Dirichlet}(\boldsymbol{\omega}|\boldsymbol{\alpha}) \propto \prod_i^K \omega_i^{\alpha_i-1} \quad (\text{S12})$$

A usual choice for the hyperparameters  $\alpha_i$  is to set them uniformly and to scale them with the number of mixtures  $K$  in the model:

$$\alpha_i = \alpha/K \quad (\text{S13})$$

For small values of  $\alpha$  (not scaling with the number of data points  $N$ , e.g.  $\alpha = 1$ ), this choice of prior has been shown to enable MCMC samplers to explore regions of parameter space with a sparse number of gaussian components, while preventing irreversible disappearance of the components during the exploration algorithm [1]. This feature is beneficial, as it allows us to select a fix number of components. The choice of priors described above has additional benefits during the sampling procedure, as will be seen in Section S4 below.

### S3.2 Nested-sampling priors

The nested sampling method explores parameter space by sampling from the prior in a constrained manner. Consequently, the convergence to the posterior distribution scales with the prior volume that is being considered. The priors chosen for the MCMC exploration described above are overly dispersed, which makes them very expensive computationally for the case of nested sampling. Computational efficiency thus requires a trade-off between a sufficiently non-informative prior and a small enough volume of the

prior space. A good compromise for the means of the mixture components can be:

$$p(x = \mu_i^T) = \begin{cases} 1 & \text{if } \min\{\mathbf{c}\} - \text{mean}(\boldsymbol{\xi}) \leq x \leq \max\{\mathbf{c}\} - \text{mean}(\boldsymbol{\xi}) \\ 0 & \text{otherwise} \end{cases} \quad (\text{S14a})$$

$$p(x = \mu_i^\xi) = \begin{cases} 1 & \text{if } \min\{\boldsymbol{\xi}\} \leq x \leq \max\{\boldsymbol{\xi}\} \\ 0 & \text{otherwise} \end{cases} \quad (\text{S14b})$$

and for the variances:

$$p(x = v_i^T) = \begin{cases} 1 & \text{if } 0 \leq x \leq s (\max\{\mathbf{c}\} - \min\{\mathbf{c}\}) \\ 0 & \text{otherwise} \end{cases} \quad (\text{S15a})$$

$$p(x = v_i^\xi) = \begin{cases} 1 & \text{if } 0 \leq x \leq s (\max\{\boldsymbol{\xi}\} - \min\{\boldsymbol{\xi}\}) \\ 0 & \text{otherwise} \end{cases} \quad (\text{S15b})$$

where  $s$  is again an expansion factor, as considered in the MCMC priors defined above. These bounds are expected contain the entire parameter space region that is relevant for the observed data sets. Since the exploration of parameter space in the nested sampling method is intensive (see next Section), we do not require to set any particular prior to the subspace of weights, which is already bounded:

$$p(\omega_i^T) = \frac{1}{K_T} \quad \forall i = 1 \cdots K_T, \quad p(\omega_i^\xi) = \frac{1}{K_\xi} \quad \forall i = 1 \cdots K_\xi \quad (\text{S16})$$

## S4 Posterior exploration

In this section, we describe the methods that we use to sample the posterior distribution given in Eq. (S5) above. Full details are given for the MCMC methods, which the nested sampling method is only commented briefly upon, since we use a standard implementation that has already been covered in many excellent papers [2, 3, 4, 5, 6].

### S4.1 MCMC sampling

The posterior distribution that we are targeting here has a complex shape that cannot be described analytically. In order to simplify the sampling procedure, we introduce a set of indicator variables  $\{\mathbf{z}^c, \mathbf{z}^\xi\}$ . The indicator variables are an auxiliary set of unobserved variables denoting the specific component of

the mixture model from which each sample has originated. They are defined as

$$\mathbf{z}_{ijk}^c = \begin{cases} 1 & \text{if } c_i \text{ comes from component } j \text{ of target and component } k \text{ of the noise} \\ 0 & \text{otherwise} \end{cases} \quad (\text{S17})$$

$$\mathbf{z}_{ij}^\xi = \begin{cases} 1 & \text{if } c_i \text{ comes from component } j \text{ of the noise} \\ 0 & \text{otherwise} \end{cases} \quad (\text{S18})$$

Thus, for each sample, the indicator variables are tensors with just one entry equal to one and the rest equal to zero. Conditioned on these variables, the mixture distributions (S3b) and (S4) can be written as

$$p(\xi_i | \phi^\xi, \mathbf{z}^\xi) = \prod_{j=1}^{K_T} (\omega_j^T \mathcal{N}(x | \mu_j^T, v_j^T))^{\mathbf{z}_{ij}^\xi} \quad (\text{S19})$$

$$p(c_i | \phi^T, \phi^\xi, \mathbf{z}^c) = \prod_{j=1}^{K_T} \prod_{k=1}^{K_\xi} \left( \omega_j^T \omega_k^\xi \mathcal{N}(c | \mu_j^T + \mu_k^\xi, v_j^T + v_k^\xi) \right)^{\mathbf{z}_{ijk}^c} \quad (\text{S20})$$

In this augmented system, the posterior distribution will be represented as,

$$\begin{aligned} p(\phi^T, \phi^\xi, \mathbf{z}^c, \mathbf{z}^\xi | \mathbf{c}, \xi) &\propto p(\mathbf{c} | \phi^T, \phi^\xi, \mathbf{z}^c) p(\xi | \phi^\xi, \mathbf{z}^T) p(\omega^T) p(\omega^\xi) = \\ &= \prod_i^{N_c} p(c_i | \phi^T, \phi^\xi, \mathbf{z}^c) \prod_j^{N_\xi} p(\xi_j | \phi^\xi, \mathbf{z}^T) p(\omega^T) p(\omega^\xi) = \\ &= \underbrace{\prod_i^{N_c} \prod_j^{K_T} \prod_k^{K_\xi} \left( \omega_j^T \omega_k^\xi \mathcal{N}(c_i | \mu_j^T + \mu_k^\xi, v_j^T + v_k^\xi) \right)^{\mathbf{z}_{ijk}^c}}_{\text{Augmented Likelihood}} \underbrace{\prod_l^{N_\xi} \prod_m^{K_\xi} \left( \omega_l^\xi \mathcal{N}(t_j | \mu_m^\xi, v_m^\xi) \right)^{\mathbf{z}_{lm}^\xi} \prod_n^{K_T} (\omega_n^T)^{\alpha_n - 1} \prod_p^{K_c} (\omega_p^\xi)^{\alpha_p - 1}}_{\text{prior}} \end{aligned} \quad (\text{S21})$$

In practice, the indicator variables are unknown and so we will have to sample from them as well as from the biological parameters. They are, however, only used as auxiliary variables to simplify the computations, and are eventually traced to produced the marginal posterior distribution.

The sampling procedure will be divided in two main phases, combining Gibbs and Metropolis steps:

#### 1. Sampling the indicator variables:

Conditioned on mixture parameters, the indicator variables are independent and their distribution has the simple form of a multinomial distribution with one draw. The convolution indicators are distributed according to

$$p(\mathbf{z}_i^c | \phi^T, \phi^\xi) = \text{Multinomial}(\mathbf{z}_i^c | n = 1, \mathbf{p}_i^c), \quad (\text{S22})$$

where the probability of each component is

$$p_{ijk}^c \propto \omega_j^T \omega_k^\xi \mathcal{N}(c_i | \mu_j^T + \mu_k^\xi, v_j^T + v_k^\xi) \quad (\text{S23})$$

Analogously, the noise indicator variables are distributed according to

$$p(\mathbf{z}_i^\xi | \phi^\xi) = \text{Multinomial}(\mathbf{z}_i^\xi | n = 1, \mathbf{p}_i^\xi), \quad (\text{S24})$$

where the probability of each component is

$$p_{ij}^\xi \propto \omega_j^\xi \mathcal{N}(\xi_i | \mu_j^\xi, v_j^\xi) \quad (\text{S25})$$

## 2. Sampling the mixture parameters:

### (a) Sampling the weights:

Conditioned on the indicator variables, the distribution of the weights takes the form of a Dirichlet distribution,

$$p(\boldsymbol{\omega}^T | \mathbf{z}^c) = \text{Dirichlet}(\boldsymbol{\omega}^T | \boldsymbol{\alpha}^T), \quad (\text{S26})$$

with parameters

$$\alpha_j^T = \sum_i^{N_c} \sum_k^{K_\xi} z_{ijk}^c + \alpha / K_\xi, \quad (\text{S27})$$

where we have included the hyperprior (S13). This choice of prior prevents a mixture from disappearing permanently, but it gives most part of the weight to the voting process of the indicator variables. An analogous expression for the weights holds for the noises:

$$p(\boldsymbol{\omega}^\xi | \mathbf{z}^c, \mathbf{z}^\xi) = \text{Dirichlet}(\boldsymbol{\omega}^\xi | \boldsymbol{\alpha}^\xi), \quad (\text{S28})$$

with parameters

$$\alpha_k^\xi = \sum_i^{N_c} \sum_j^{K_T} z_{ijk}^c + \sum_i^{N_\xi} z_{ik}^\xi + \alpha / K_\xi \quad (\text{S29})$$

### (b) Sampling the variances:

The means and the variances of the two datasets (target and noise) are entangled due to the convolution. Moreover, no simple marginal expression exists for the distribution of the variances. Hence, a slice-sampling algorithm [7] is used in order to make a new proposal for each variance. This algorithm is composed of the following steps (in all the equations that follow, the rest of the parameters are not mentioned for sake of simplicity):

- i. First, we need to choose a starting value of the probability density of each variance. The standard choice in slice sampling implementations [7] is:

$$p^* = p(v_j) * \text{Uniform}(0, 1) \quad (\text{S30})$$

Here we cannot use directly this expression, however, because we do not have a normalized expression for the variances. We thus use the marginal posterior likelihood:

$$\log p^* = \bar{L} + \log \text{Uniform}(0, 1) \quad (\text{S31})$$

For the target variances, this likelihood takes the form

$$\bar{L}^c(v_j^T) = \prod_i^{N_c} \prod_k^{K_\xi} \left( \mathcal{N}(c_i | \mu_j^T + \mu_k^\xi, v_j^T + v_k^\xi) \right)^{z_{ijk}^c} \Gamma(v_j^T | \theta_{\text{prior}}^T, k_{\text{prior}}^T) \quad (\text{S32})$$

and for the noise variances, the corresponding expression is

$$\bar{L}^\xi(v_k^\xi) = \prod_i^{N_c} \prod_j^{K_T} \left( \mathcal{N}(c_i | \mu_j^T + \mu_k^\xi, v_j^T + v_k^\xi) \right)^{z_{ijk}^c} \prod_l^{N_\xi} \left( \mathcal{N}(t_j | \mu_m^\xi, v_m^\xi) \right)^{z_{lm}^\xi} \Gamma(v_j^\xi | \theta_{\text{prior}}^\xi, k_{\text{prior}}^\xi) \quad (\text{S33})$$

- ii. Next we expand the slice by looking first for a new slice minimum, choosing  $v_{\min}^* = v_j - nh$ , setting initially  $n = 1$  and an arbitrary  $h > 0$ . If  $\bar{L}(v_{\min}^*) < \log p^*$  we accept draw, otherwise we increase  $n$  in 1 unit and repeat the process by choosing a new minimum slice  $v_{\min}^*$  until the draw is accepted. Next we perform a similar expansion to identify a new slice maximum.
- iii. Next we sample from the slice, by setting  $v_{\text{prop}}^* = \text{Uniform}(v_{\min}^*, v_{\max}^*)$ . If  $p(v_{\text{prop}}^*) > p^*$  we accept the draw ( $v_{j,\text{new}} = v_{\text{prop}}^*$ ). Otherwise, if  $v_{\text{prop}}^* < v_j$ , we update the minimum ( $v_{\min}^* = v_{\text{prop}}^*$ ). Alternatively, if  $v_{\text{prop}}^* > v_j$ , we update the maximum ( $v_{\max}^* = v_{\text{prop}}^*$ ). We then choose a new value of  $v_{\text{prop}}^*$  and repeat the process until a draw is accepted.

This method is computationally more expensive than a Metropolis algorithm, but it has the benefit of not depending on the correct tuning of parameters to avoid an excess of rejection steps. This is preferable in our case, since our parameters may have very different scales and a correct tuning is unfeasible.

(c) Sampling the means:

Conditioned on the rest of the parameters, the means can be easily sampled. We now describes all the steps of the process (as before, in all the equations that follow, the rest of the parameters are not mentioned for sake of simplicity).

i. For the target parameters, the means can be sampled from normal distributions:

$$p(\mu_j^T) = \mathcal{N}(\mu_j^T | \mu_{j,\text{eff}}^T, v_{j,\text{eff}}^T), \quad (\text{S34})$$

where the effective mean is

$$\mu_{j,\text{eff}}^T = \frac{\sum_i^{N_c} \sum_k^{K_\xi} \frac{c_i + \mu_k^\xi}{v_j^T + v_k^\xi} + \frac{\mu_{\text{prior}}^T}{v_{\text{prior}}^T}}{\sum_i^{N_c} \sum_k^{K_\xi} \frac{1}{v_j^T + v_k^\xi} + \frac{1}{v_{\text{prior}}^T}} \quad (\text{S35})$$

and the effective variance is

$$v_{j,\text{eff}}^T = \frac{1}{\sum_i^{N_c} \sum_k^{K_\xi} \frac{1}{v_j^T + v_k^\xi} + \frac{1}{v_{\text{prior}}^T}} \quad (\text{S36})$$

ii. For the noise, similar expressions hold:

$$p(\mu_j^\xi) = \mathcal{N}(\mu_j^\xi | \mu_{j,\text{eff}}^\xi, v_{j,\text{eff}}^\xi) \quad (\text{S37})$$

where the effective mean is

$$\mu_{k,\text{eff}}^\xi = \frac{\sum_i^{N_c} \sum_j^{K_T} \frac{c_i + \mu_k^\xi}{v_j^T + v_k^\xi} + \sum_i^{N_\xi} \frac{\xi_i}{v_k^\xi} + \frac{\mu_{\text{prior}}^\xi}{v_{\text{prior}}^\xi}}{\sum_i^{N_c} \sum_j^{K_T} \frac{1}{v_j^T + v_k^\xi} + \sum_i^{N_\xi} \frac{1}{v_k^\xi} + \frac{1}{v_{\text{prior}}^\xi}} \quad (\text{S38})$$

and the effective variance is

$$\sigma_{k,\text{eff}}^\xi = \frac{1}{\sum_i^{N_c} \sum_j^{K_T} \frac{1}{v_j^T + v_k^\xi} + \sum_i^{N_\xi} \frac{1}{v_k^\xi} + \frac{1}{v_{\text{prior}}^\xi}} \quad (\text{S39})$$

#### S4.1.1 Default initial conditions for the sampling

As described above, our method uses a combination of Gibbs and slice sampling. In order to initialize the parameters close to a solution, it is common to use a Expectation Maximization algorithm. However, in our case there is no closed form for the steps of the expectation maximization. Therefore, as an alternative we initialize the algorithm by using K-means clustering [8]. This method is adequate for small noises, as the dataset is expected to be distributed around the modes of the target distribution. On the other hand, MCMC may fail to explore adequately the posterior space in situations with high amounts of noise, as mentioned above.

### S4.1.2 Sampling identifiability and assessment

When using the MCMC method to draw samples from a posterior distribution, it is necessary to assess that the sampling is representative of the distribution. This may be done by the inspection of the several independent realizations of the chains. However, mixtures models are unidentifiable when they are symmetric under label exchange of the different components, unless there is an asymmetric informative prior to remove the degeneracy. This might cause difficulties when checking the convergence of the chains. In order to mitigate this problem, it is usually convenient to sort the draws of the traces in two ways:

1. By the weight of each component. This leads to traces sorted in increasing order of contribution to the mixture.
2. By the position of the mean. This can be useful in situations where two or more components have a similar contribution.

In order to assist the visual inspection of the convergence, it is convenient to check the mixing of the chains using the ratio of the sequence variance between and within chains ( $\hat{R}$ ). This ratio measures how the variance changes during sampling and between samples. A value close to 1 indicates that the sample is well mixed, whereas values far from 1 indicated the need of performing more sampling steps to reach convergence.

Even if the chain is well mixed, the correlation between MCMC samples might lead to a poor representation of the posterior distribution. The specific number of steps of the algorithm needed to produce independent samples (effective samples) will be case dependent. Another important feature is the number of effective samples  $n_{\text{eff}}$  needed to recapitulate the posterior distribution for a given parameter. As a rule of thumb, we consider in our case that  $n_{\text{eff}} = 100$  samples resolve the posterior distribution adequately.

## S4.2 Nested sampling

This approach to exploring the posterior distribution is based on sampling from the prior distribution and evaluating the likelihood in a nested-constrained manner. There is a large number of articles that describe the process of nested sampling very clearly [2, 3, 4, 5, 6], so here we only mention the key aspects of the procedure.

The nested sampling (NS) idea was initially developed to compute the evidence of Bayesian models by

evaluating the integral

$$\text{Evidence}(H|\{x\}) = \int \mathcal{L}(\{x\}|\theta, H)p(\theta, H)d\theta \quad (\text{S40})$$

where  $\{x\}$  is the data,  $H$  is the model being tested,  $\theta$  represents the parameters of the model. This integral quantifies the evidence of a model explaining the data. This score can be compared between models in order to perform model selection. The NS is a stochastic method for evaluating this integral, and gives as a by-product a representative sample set of the posterior distribution.

In recent years, many refinements have been introduced in this method, that lead to more representative posterior samples and enable exploring complex and highly degenerate posterior distributions, even in high dimensions. This makes nested sampling a very appropriate method to address the deconvolution problem.

### S4.3 Sampler selection

The two sampling methods discussed above (MCMC and nested sampling) share the goal of sampling from the posterior distribution. However, they each have unique characteristics:

- The MCMC sampler has fast convergence in regions close to a minimum of the posterior distribution. This allows short computation times. Moreover, the choice of the Dirichlet prior gives us the additional advantage of obtaining sparse solutions in the number of components, which further helps in the process of component selection for the model. These characteristics make the MCMC sampler a suitable choice for exploratory analysis of the deconvolution. The main drawback of the sampler is that the deconvolution problem usually has complex posterior landscapes with high degeneracy and multimodality. In such context it is common for the sampler to get stuck in some regions of parameter space, with very sparse jumps between modes, which makes it computationally hard to reach a proper convergence to the real posterior distribution.
- The nested sampler and its posterior refinements overcome the problem of exploring the above-mentioned complex regions of parameter space by relying in a different way of sampling. Although in its current state, our NS model cannot select on its own the number of components, it can potentially be used for model selection by comparing the evidence between different realizations of the model with different conditions. The main drawback of this approach is that it is computationally more expensive, with the computational time increasing exponentially with the dimensionality of the problem.

Considering the benefits and drawbacks of both methods, we find that their combination is the optimal solution for a proper analysis of the deconvolution:

- Use MCMC with a relatively high number of components for both the noise and the target, and check the posterior distributions to see how many components are representative.
- Use NS with the number of components obtained during the MCMC run as a sparse (and reasonable) starting point.

As an additional step, if the deconvolution does not seem satisfactory, we can increase one by one the number of components until the evidence reaches a maximum.

## S5 Modifications for the gamma basis

Small differences have to be implemented when using a basis of gamma functions. Specifically, for the target and noise distributions:

$$p(T|\phi^T = \{\omega^T, \theta^T, k^T\}) = \sum_{i=1}^{K_T} \omega_i^T \Gamma(x|\theta_i^T, k_i^T) \quad (\text{S41})$$

$$p(\xi|\phi^\xi = \{\omega^\xi, \theta^\xi, k^\xi\}) = \sum_{i=1}^{K_\xi} \omega_i^\xi \Gamma(\xi|\theta_i^\xi, k_i^\xi), \quad (\text{S42})$$

where the gamma distribution is defined as

$$\Gamma(x|\theta, k) = \frac{1}{\Gamma(k)\theta^k} x^{k-1} e^{-\frac{x}{\theta}}, \quad (\text{S43})$$

with  $\Gamma(k)$  denoting the gamma function.

The main problem of using gamma basis functions is that the convolution of two gammas does not have a simple closed solution. Exact solutions exist, as derived by [9, 10] but they are computationally infeasible for the purposes of the posterior exploration. Instead, we use an approximation in terms of matching moments. This approximation has been shown to be appropriate for most parameter combinations. Using this approximation,

$$p(c|\phi^T, \phi^\xi) \approx \sum_{i=1}^{K_T} \sum_{j=1}^{K_\xi} \omega_j^T \omega_j^\xi \Gamma(c|\theta_{ij}^{\text{eff}}, k_{ij}^{\text{eff}}), \quad (\text{S44})$$

where the effective parameters are defined by

$$\theta_{ij}^{\text{eff}} = \frac{(\theta_i^T)^2 k_i^T + (\theta_j^\xi)^2 k_j^\xi}{\theta_i^T k_i^T + \theta_j^\xi k_j^\xi} \quad (\text{S45a})$$

$$k_{ij}^{\text{eff}} = \frac{(\theta_i^T k_i^T + \theta_j^\xi k_j^\xi)^2}{(\theta_i^T)^2 k_i^T + (\theta_j^\xi)^2 k_j^\xi} \quad (\text{S45b})$$

As for the priors, given that the parameters of the gamma distributions are positive defined, we consider that they follow gamma distributions themselves:

$$p(\theta_i^T) = \Gamma(\theta_i^T | \theta_{\theta, \text{prior}}^T, k_{\theta, \text{prior}}^T) \quad (\text{S46a})$$

$$p(\theta_i^\xi) = \Gamma(\theta_i^\xi | \theta_{\theta, \text{prior}}^\xi, k_{\theta, \text{prior}}^\xi) \quad (\text{S46b})$$

$$p(k_i^T) = \Gamma(k_i^T | \theta_{k, \text{prior}}^T, k_{k, \text{prior}}^T) \quad (\text{S46c})$$

$$p(k_i^\xi) = \Gamma(k_i^\xi | \theta_{k, \text{prior}}^\xi, k_{k, \text{prior}}^\xi) \quad (\text{S46d})$$

We select the hyperpriors based again in heuristic arguments:

$$\theta_{\theta, \text{prior}}^T = s \sqrt{\frac{\text{var}(\mathcal{D}_{\text{signal}})}{\text{mean}(\mathcal{D}_{\text{signal}})}} \quad (\text{S47a})$$

$$\theta_{\theta, \text{prior}}^\xi = s \sqrt{\frac{\text{var}(\mathcal{D}_{\text{noise}})}{\text{mean}(\mathcal{D}_{\text{noise}})}} \quad (\text{S47b})$$

$$\theta_{k, \text{prior}}^T = s \sqrt{\frac{\text{mean}(\mathcal{D}_{\text{signal}})^2}{\text{var}(\mathcal{D}_{\text{signal}})}} \quad (\text{S47c})$$

$$\theta_{k, \text{prior}}^\xi = s \sqrt{\frac{\text{mean}(\mathcal{D}_{\text{noise}})^2}{\text{var}(\mathcal{D}_{\text{noise}})}} \quad (\text{S47d})$$

$$k_{\theta, \text{prior}}^T = k_{\theta, \text{prior}}^\xi = k_{k, \text{prior}}^T = k_{k, \text{prior}}^\xi = 1.1 \quad (\text{S47e})$$

Here  $\mathcal{D}_{\text{signal}}$  and  $\mathcal{D}_{\text{noise}}$  represent the measurement dataset of the total signal and the noise, respectively. In the expressions above, we choose a conservative value for the factor  $s = 10$ . The square root allows us to limit the exploration of the corresponding space, by reducing the overall expected maximum while keeping a vague value around the expected gamma distribution.

In the case of nested sampling, using the same prior usually leads to a proper exploration of parameter space. An alternative solution is to use uniform prior distributions between zero and the theta values defined in Eqs. (S47), as upper limits for the different parameters.

Finally, for the MCMC sampler, no analytic expression is available to sample the parameters of gamma basis. Therefore, after sampling the indicator variables and the weights, slice sampling is used for both the  $\theta$  and  $k$  parameters, as described in Sec. S4.1.

## S6 Efficiency assessment

So far, the efficiency of deconvolution methods has been assessed using quantifiers applicable to point estimates, which are the ones proposed in the literature to date. To compare the efficiency of our model with previous methods that do not obey the positivity nor the normalization conditions, we can use the Mean Integrated Squared Estimation (MISE) measure:

$$\text{MISE} = \int_{-\infty}^{\infty} (p_{\text{true}}(x) - p_{\text{est}}(x))^2 dx, \quad (\text{S48})$$

where  $p_{\text{true}}$  is the real target distribution and  $p_{\text{est}}$  is the point estimate of the deconvolved distribution. This is the traditional measure of convergence, but it is hard to interpret as it only has a lower bound. To address this issue, we introduce the mean integrated overlap (MIO):

$$\text{MIAE} = 1 - \frac{1}{2} \int_{-\infty}^{\infty} |p_{\text{true}}(x) - p_{\text{est}}(x)| dx \quad (\text{S49})$$

This measure has the property that it is bounded in the interval  $[0, 1]$  if the true and the estimated distributions are normalized, with 0 corresponding to the case of no overlap between distributions, and 1 to the case of complete overlap. Values below zero can be obtained if the estimated distribution does not follow the positivity requirement nor the normalization condition, as it is the case in FFT-based deconvolutions.

## References

- [1] Gelman A, Carlin JB, Stern HS, Dunson DB, Vehtari A, Rubin DB. Bayesian Data Analysis, Third Edition. Taylor & Francis; 2013. Available from: <https://books.google.es/books?id=ZXL6AQAAQBAJ>.
- [2] Skilling J. Nested sampling for general Bayesian computation. Bayesian Analysis. 2006;1(4):833–859. Available from: <https://doi.org/10.1214/06-BA127>.
- [3] Feroz F, Hobson MP. Multimodal nested sampling: an efficient and robust alternative to Markov Chain Monte Carlo methods for astronomical data analyses. Monthly Notices of the Royal Astronomical Society. 2008;384(2):449–463. Available from: <https://doi.org/10.1111/j.1365-2966.2007.12353.x>.
- [4] Brewer BJ, Pártay LB, Csányi G. Diffusive Nested Sampling. Statistics and Computing. 2011;21(4):649–656. Available from: <https://doi.org/10.1007/s11222-010-9198-8>.

- [5] Higson E, Handley W, Hobson M, Lasenby A. Dynamic nested sampling: an improved algorithm for parameter estimation and evidence calculation. *Statistics and Computing*. 2019;29(5):891–913. Available from: <https://doi.org/10.1007/s11222-018-9844-0>.
- [6] Speagle JS. dynesty: a dynamic nested sampling package for estimating Bayesian posteriors and evidences. *Monthly Notices of the Royal Astronomical Society*. 2020;493(3):3132–3158. Available from: <https://doi.org/10.1093/mnras/staa278>.
- [7] Neal RM. Slice sampling. *The annals of statistics*. 2003;31(3):705–767. Available from: <https://doi.org/10.1214/aos/1056562461>.
- [8] Hastie T, Tibshirani R, Friedman JH. *The elements of statistical learning*. Springer; 2009. Available from: <https://link.springer.com/book/10.1007/978-0-387-84858-7>.
- [9] Moschopoulos PG. The distribution of the sum of independent gamma random variables. *Annals of the Institute of Statistical Mathematics*. 1985;37:541–544. Available from: <https://doi.org/10.1007/BF02481123>.
- [10] Barnabani M. An approximation to the convolution of gamma distributions. *Communications in Statistics - Simulation and Computation*. 2017;46:331–343. Available from: <https://doi.org/10.1080/03610918.2014.963612>.

## Supplementary figures

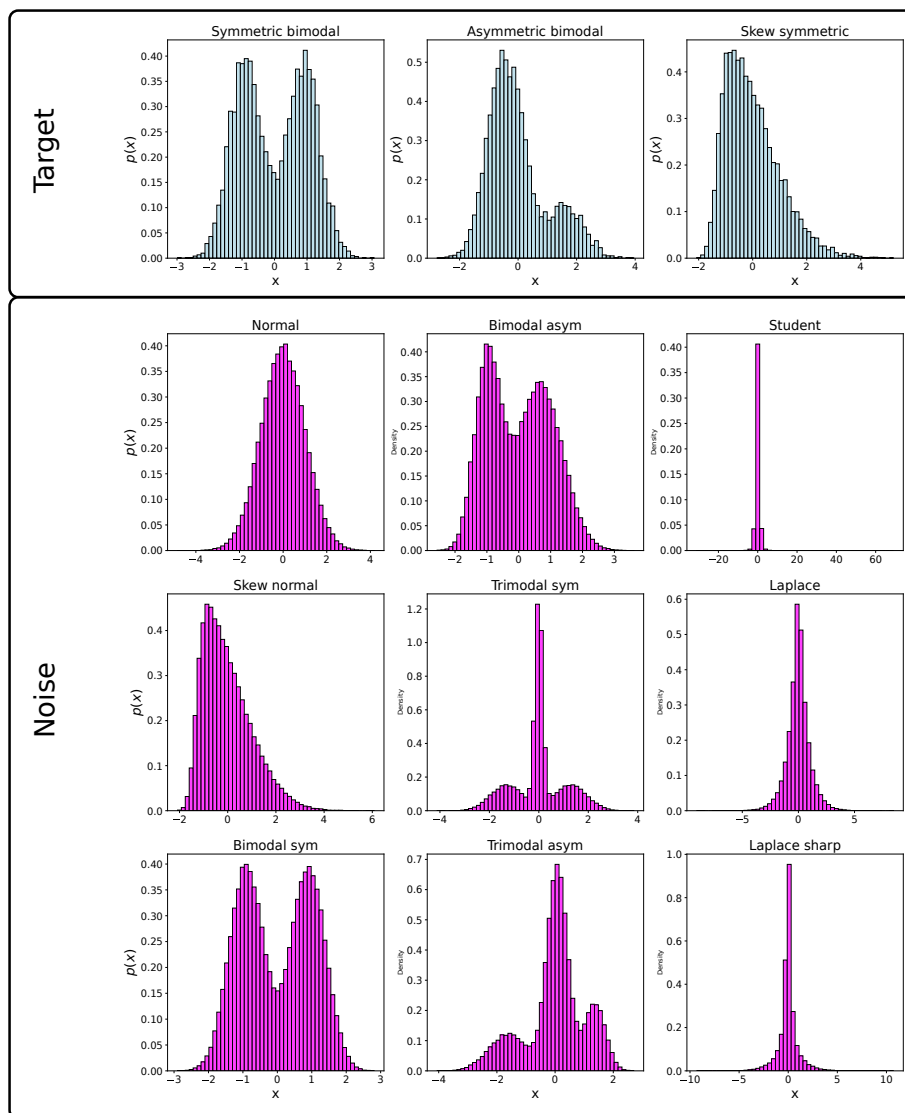

Figure S1: Synthetic target (top row) and noise (3 bottom rows) distributions.

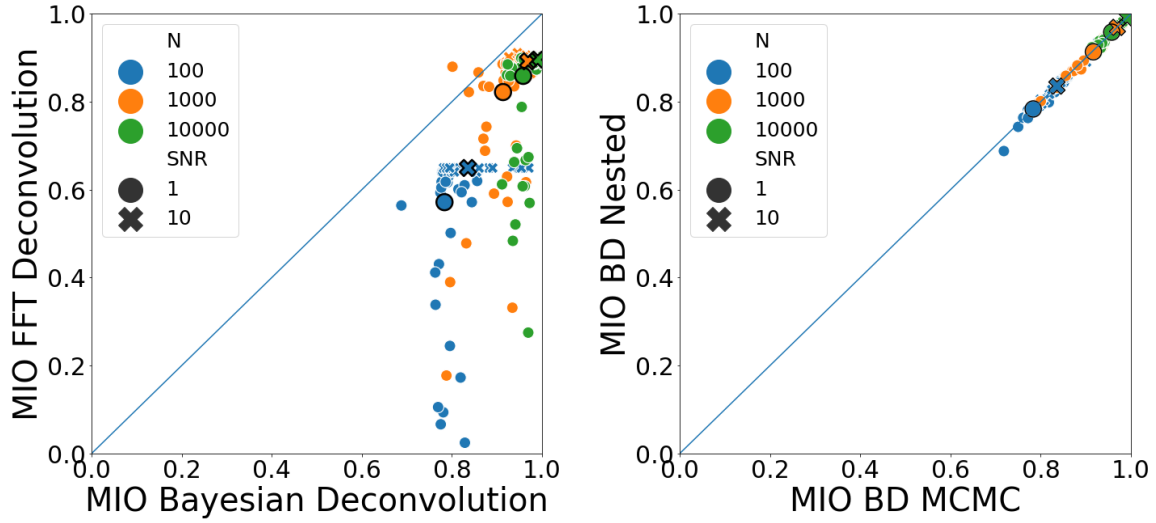

Figure S2: Similarity between the deconvolved and ground-truth target distributions as expressed by the Mean Integrated Overlap (MIO) for the two sampling methods (x and y axis, right panel) being used with our Bayesian deconvolution algorithm. The left panel, replotted from Fig. 3 in the main text for easy reference, shows a comparison between our method with MCMC sampling (x-axis) and a Fourier-based method (y axis). Colors represent different sampling sizes for the synthetic datasets described in the main text, with  $\text{SNR} = 1$  (circles) and  $\text{SNR} = 10$  (crosses). The large symbols represent the mean MIO over the different samples for each sample size and SNR.

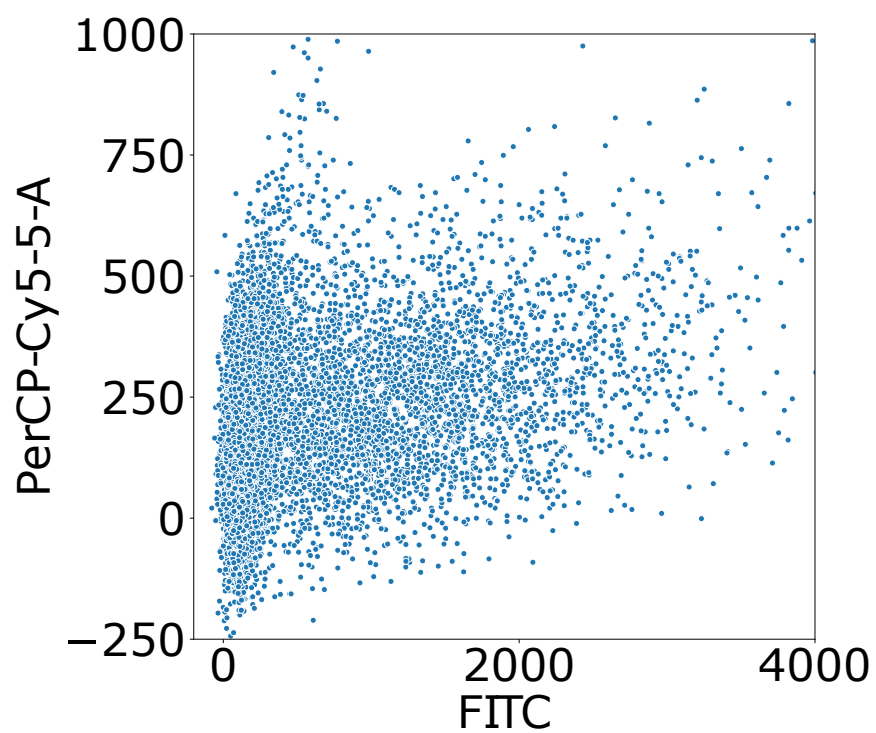

Figure S3: Scatter plot of the fluorescence signals coming from the target fluorophore (x axis) and the dye (y axis) representing the noise signal, for the analysis discussed in Sec. III.B of the main text. Every symbol in the figure corresponds to one cell.

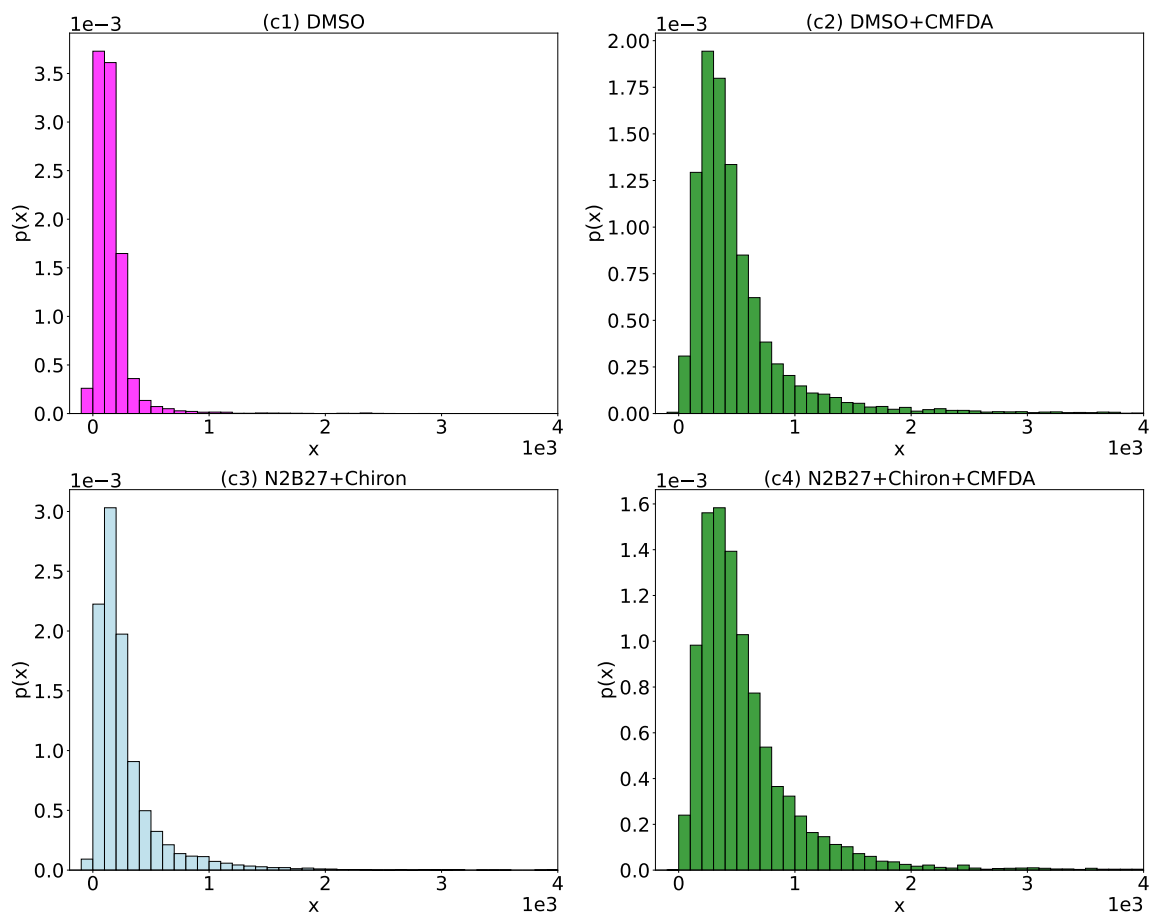

Figure S4: Flow cytometry distributions obtained in the four experimental conditions discussed in Sec. III.C of the main text.
